# Supplementary material for: Covert Channel-Based Transmitter Authentication in Controller Area Networks
Source: arXiv:1912.04735 source file (2019-12-08)
Supplement: Supplementary file 1 [file appendices.tex]

\newpage

\balance
\appendices
% \section{CAN Frame}
% \label{appendix:CAN_frame}
% As illustrated in Figure~\ref{fig:can_frame_structure}, each CAN frame or message has a set of predefined fields, including the Start of Frame (SOF) field, the Arbitration field (including a 11-bit message ID for the base frame format or a 29-bit message ID for the extended frame format), the Control field, the Data field (8-64 bits), the CRC field, the ACK field, and the End of Frame (EOF) field.

% \begin{figure}[ht!]
% \centering
% \includegraphics[width=1\columnwidth]{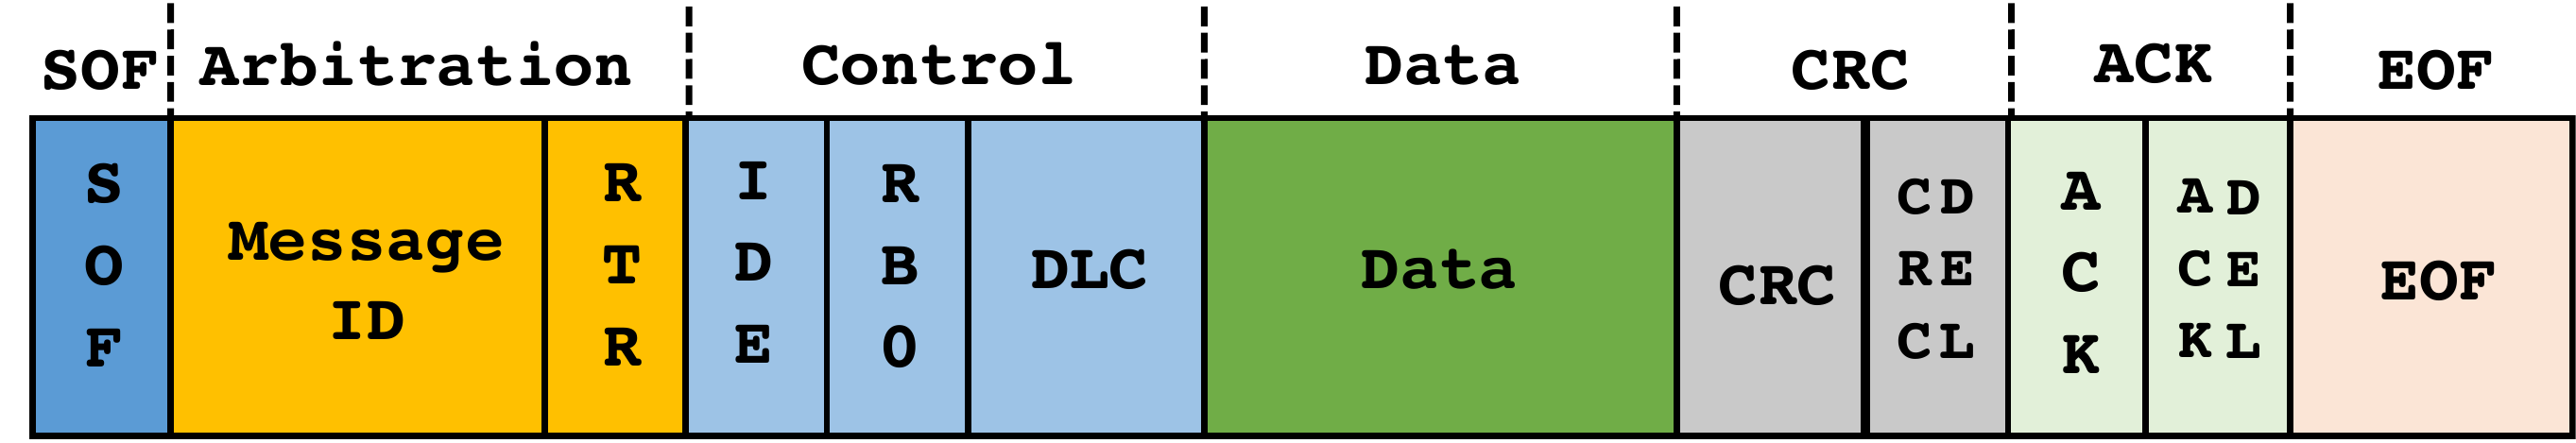}
% \caption{Illustration of CAN frame structure.}
% \label{fig:can_frame_structure}
% \vspace{-0.3cm}
% \end{figure}

\section{Impact on CAN Bus Schedulability}
\label{appendix:schedulability}
In order to understand the impact of the timing parameter $\delta$ introduced by the IAT-based covert channel in TACAN on CAN bus schedulability, we apply the schedulability analysis in \cite{davis2007controller}.
For the ease of discussion, we provide a summary of definitions as below. 
%The same notations in \cite{davis2007controller} are used for consistency.
\begin{itemize}
    \item $k$: Message priority, which is used interchangeably with the message ID.
    \item $C_k$: Transmission time, defined as the longest time that the message can take to be transmitted.
    \item $J_k$: Queuing jitter, defined as the longest time between the initiating event and the message being queued, ready to be transmitted on the bus.
    \item $w_k$: Queuing delay, defined as the longest time that the message can remain in the CAN controller slot or device driver queue, before commencing successful transmission on the bus.
    \item $T_k$: Message period, defined as the minimum inter-arrival time of the event that triggers queueing of the message. 
    Such events may occur strictly periodically with a period of $T_k$ or sporadically with a minimum separation of $T_k$. 
    \item $R_k$: Worst-case response time of message $k$, defined as the longest time from the initiating event occurring to the message being received by the nodes that require it.
    \item $D_k$: Hard deadline, defined as the maximum permitted time from occurrence of the initiating event to the end of successful transmission of the message. 
\end{itemize}
A message is \textit{schedulable} if and only if its worst-case response time is no greater than its deadline ($R_k \leq D_k$). 
A CAN bus is schedulable if and only if all messages on the CAN bus are schedulable.

As per \cite{davis2007controller}, we have $C_k = (80 + 10 s_k)\tau_{bit}$ (including bit stuffing), where $s_k$ is the number of data bytes and $\tau_{bit}$ is the transmission time of a single bit. 
For a $8$-byte message on a $500$ kbps CAN bus, we have $\tau_{bit}=2~\mu$s and  $C_k=320$ $\mu$s.
While CAN nodes typically have separate clock sources, all the timing quantities (e.g., message jitters, bit times, message periods, and deadlines) that derived from node clocks will be converted to real-time. 

The message $k$'s worst-case response time $R_k$ is given by
\begin{equation*}
    R_k = J_k + w_k + C_k,
\end{equation*}
and the queuing delay $w_k$ consists of two elements:
\begin{itemize}
    \item \textit{Blocking} $B_k$, due to lower priority messages  being transmitted when message $k$ is queued, and
    \item \textit{Interference} due to higher priority messages which may win arbitration and be transmitted in preference to message $k$.
\end{itemize}
The blocking delay is given by $B_k = \max_{i \in lp(k)} (C_i)$, where $lp(k)$ is the set of messages with lower priority than $k$.

In order to analyze the worst-case response time, it is important to characterize the busy period, where all messages of priority $k$ or higher, queued strictly before the end of busy period, are transmitted during the busy period. 
The maximal busy period begins with a so-called critical instant where message $k$ is queued simultaneously with all higher priority messages and then each of these higher priority messages is subsequently queued again after the shortest possible time interval.

For simplicity, we assume that only one instance of message $k$ is transmitted during a priority level-$k$ busy period. 
In this case, the worst-case queuing delay is 
\begin{equation}\label{eq:worst_case_queuing_delay}
    w_k = B_k + \sum_{\forall i \in hp(k)} \left\lceil \frac{w_k + J_i + \tau_{bit}}{T_i}  \right\rceil C_i.
\end{equation}
Since the right hand side is a monotonic non-decreasing function of $w_k$, Eq.~(\ref{eq:worst_case_queuing_delay}) can be solved using the following recurrence relation,
\begin{equation}\label{eq:worst_case_queuing_delay2}
    w_k^{n+1} = B_k + \sum_{\forall i \in hp(k)} \left\lceil \frac{w_k^n + J_i + \tau_{bit}}{T_i} \right\rceil C_i.
\end{equation}
A suitable starting value is $w_k^0 = B_k$, and the recurrence relation iterates until, either $J_k + w_k^{n+1} + C_k > D_k$, i.e., the message is not schedulable, or $w_k^{n+1}=w_k^n$, in which case the worst-case response of message $k$ is given by $J_k + w_k^{n+1}+C_k$. 

In order to apply the above schedulability analysis to TACAN, we define $T'_k = T_k - \delta$. 
Since TACAN adds at most $\delta$ to each ITT, which can be considered as part of the queuing jitter, we have $J'_k=J_k + \delta$. 
Assume that $\delta = 0.01 T_k$ and all messages employ the IAT-based covert channel. 
By substituting $T'_k=0.99 T_k$ and $J'_m=J_m + 0.01 T_k$ into Eq.~(\ref{eq:worst_case_queuing_delay2}), we have
\begin{align}
    w_k^{' n+1} &= B_k + \sum_{\forall i \in hp(k)} \left\lceil \frac{w_k^{' n} + (J_i + 0.02 T_i) + \tau_{bit}}{0.98 T_i} \right\rceil C_i \nonumber\\
    &\approx B'_k  + 
    \sum_{\forall i \in hp(k)} \left\lceil \frac{w_k^{' n} + J_k + \tau_{bit}}{T_i} \right\rceil C'_i, \label{eq:updated_worst_case_queuing_delay}
\end{align}
where 
\begin{equation}\label{eq:appendix:blocking_delay}
    B_k' = B_k + \sum_{\forall i \in hp(k)} \left(\frac{0.01}{0.99} C_i \right), 
\end{equation}
and 
\begin{equation}\label{eq:appendix:msg_tx_time}
    C'_i = \frac{1}{0.99} C_i = 1.01 C_i.
\end{equation}
Therefore, the impact of $\delta$ on the worst-case response time is threefold: 1) increasing the queuing jitter by a fixed amount of time, 2) increasing the blocking delay by a bounded amount of time, and 3) increasing the equivalent message transmission time of higher priority messages by a certain percentage.

As an example, let us consider a 10-ms message and set $\delta=0.01T=0.1$ ms. 
Then the increase in the queuing jitter is $100~\mu$s. 
Assuming 45 higher priority messages (half of the messages on the EcoCAR \cite{ecocar}) with 8-byte data on a 500 kbps bus ($C_i=320~\mu$s), the increase in the blocking delay is $145~\mu$s (Eq.~(\ref{eq:appendix:blocking_delay})). 
In addition, the equivalent increase in the message transmission time of each higher priority message is $1\%$, which is equal to $3.2~\mu$s (Eq.~(\ref{eq:appendix:msg_tx_time})). 
By solving Eq.~(\ref{eq:updated_worst_case_queuing_delay}), we can compute the corresponding worst-case response time of message $k$ with TACAN. 
%The above discussion suggests that schedulability tests will need to be performed during TACAN configurations to ensure the schedulability of the system.
Hence, to achieve effective use of covert channels, the TACAN parameter $\delta$ needs to be experimentally obtained and fine tuned prior to deployment to ensure the schedulability of the CAN bus.
